# Supplementary material for: A Bisimilarity Congruence for the Applied pi-Calculus Sufficiently Coarse to Verify Privacy Properties
Source: arXiv:1811.02536 source file (2018-11-06)
Supplement: Supplementary file 1 [file appendix.tex]

\section*{Appendix}

%\begin{definition}
%We say a history $h$ grounds proceses $P$, $Q \hdots$, whenever: all free variables in $P, Q, \hdots$ appear as outputs in $h$.
% and there are at least as many fresh outputs in $h$ as there are input actions in $P$ and $Q$.
%\end{definition}

\begin{lemma}\label{lemma:transition}
Assume history $h$ grounds $P$.
We have $h \colon P \lts{\pi} Q$ according to Fig.~\ref{figure:pi},
iff $P \lts{\pi} Q$ in the classical $\pi$-calculus labelled transition system~\cite{Parrow1995}.
\end{lemma}

%Note by $P \lts{\pi} Q$ in the classical $\pi$-calculus labelled transition system with mismatch~\cite{Parrow1995}, we mean a labelled transition according to Fig.~\ref{figure:classic-lts}, where $x \not= y$ holds whenever $x$ and $y$ are distinct, since classical late bisimulation assumes free variables are distinct names (constants).

For this closed labelled transitions the following definition of late bisimulation is standard.
\begin{definition}[late bisimulation]
A symmetric relation $\mathrel{\mathcal{R}}$ is a late bisimulation whenever,
if $P \mathrel{\mathcal{R}} Q$, then:
\begin{itemize}
\item If $P \lts{\alpha} P'$ then there exists $Q'$ such that $Q \lts{\alpha} Q'$ and $P' \mathrel{\mathcal{R}} Q'$, where $\alpha$ is of the form $\tau$ or $\co{M}N$.
\item If $P \lts{M(x)} Q'$, where $x$ fresh for $P$ and $Q$, then there exists $Q'$ such that $Q \lts{M(x)} Q'$ and 
for all messages $N$, $P'\sub{x}{N} \mathrel{\mathcal{R}} Q'\sub{x}{N}$.
\item If $P \lts{\co{M}(x)} P'$, where $x$ fresh for $P$ and $Q$, then there exists $Q'$ such that $Q \lts{\co{M}(x)} Q'$ and $P' \mathrel{\mathcal{R}} Q'$.
\end{itemize}
Late bisimilarity is the greatest late bisimulation.
Strong equivalence is the greatest congruence contained in late bisimilarity.
\end{definition}

\begin{figure}[h!]
\[
\begin{gathered}
\begin{array}{c}
\begin{prooftree}
\bn{\pi} \cap \fv{\pi} = \emptyset
\justifies
\mathopen{\pi.}P \lts{\pi} P
%\using\mbox{\textsc{Act}}
\end{prooftree}
\qquad
\begin{prooftree}
P \lts{\co{M}x} Q
\quad
x \not\in \fv{M}
\justifies
\nu x.P \lts{\co{M}(x)} Q
%\using\mbox{\textsc{Open}}
\end{prooftree}
\qquad
\begin{prooftree}
P \lts{\pi} Q
\quad
M \not= N
\justifies
 {\mathopen{\left[M \not= N\right]}{P}\lts{\pi}{Q}}
%\using\mbox{\textsc{Mismatch}}
\end{prooftree}
\\[15pt]
\begin{prooftree}
P \lts{\pi} Q
\justifies
{\mathopen{\left[M=M\right]}{P}\lts{\pi}{Q}}
\end{prooftree}
\qquad
\begin{prooftree}
 P \lts{\pi} Q
\quad
x \not\in \mathrm{n}(\pi)
\justifies
 {{\nu x.P}\lts{\pi}{\nu x.Q}}
%\using\mbox{\textsc{Res}}
\end{prooftree}
\qquad
\begin{prooftree}
 {P \lts{\pi} Q}
\quad
\fv{R} \cap \bn{\pi} = \emptyset
\justifies
 {{P \cpar R} \lts{\pi} {Q \cpar R}}
%\using \mbox{\textsc{Par-l}}
\end{prooftree}
\\[15pt]
\begin{prooftree}
 P \lts{\pi} R
\justifies
 P + Q \lts{\pi} R
%\using\mbox{\textsc{Sum-l}}
\end{prooftree}
\qquad
\begin{prooftree}
 P \lts{\co{M}(x)} P'
\quad
 Q \lts{M(x)} Q'
\justifies
 {P \cpar Q}\lts{\tau}{\mathopen{\nu x.}\left(P' \cpar Q'\right)} 
%\using \mbox{\textsc{Close-l}}
\end{prooftree}
\qquad
\begin{prooftree}
 P \lts{\co{M}N} P'
\quad
 Q \lts{M(x)} Q'
%\quad x \not\in\fv{A}
\justifies
 {P \cpar Q}\lts{\tau} P' \cpar Q'\sub{x}{N}
%\using \mbox{\textsc{Comm-l}}
\end{prooftree}
\end{array}
\end{gathered}
\]
\caption{
The classical late transition semantics for the finite $\pi$-calculus
with mismatch~\cite{Parrow1995},
where mismatch implicitly assumes messages are grounded.
}\label{figure:classic-lts}
\end{figure}

\begin{comment}
\begin{definition}[late bisimulation]
A symmetric relation $\mathrel{\mathcal{R}}$ is a late bisimulation whenever,
if $P \mathrel{\mathcal{R}} Q$, then:
\begin{itemize}
\item If $P \lts{\alpha} P'$ then there exists $Q'$ such that $Q \lts{\alpha} Q'$ and $P' \mathrel{\mathcal{R}} Q'$, where $\alpha$ is of the form $\tau$ or $\co{M}N$.
\item If $P \lts{M(x)} Q'$, where $x$ fresh for $P$ and $Q$, then there exists $Q'$ such that $Q \lts{M(x)} Q'$ and 
for all messages $N$, $P'\sub{x}{N} \mathrel{\mathcal{R}} Q'\sub{x}{N}$.
\item If $P \lts{\co{M}(x)} P'$, where $x$ fresh for $P$ and $Q$, then there exists $Q'$ such that $Q \lts{\co{M}(x)} Q'$ and $P' \mathrel{\mathcal{R}} Q'$.
\end{itemize}
Late bisimilarity is the greatest late bisimulation.
Late congruence is the greatest congruence contained in late bisimilarity.
\end{definition}
\end{comment}

\begin{lemma}\label{lemma:transition-names}
The following properties hold for the $\pi$-calculus:\ross{Perhaps include contexts.}
\begin{itemize}
\item If $P \lts{\co{x}(z)} Q$ then 
then $\fv{Q} \subseteq \fv{P} \cup \left\{ x \right\}$.
\item
If $P \lts{x(z)} Q$ then $\fv{Q} \subseteq \fv{P} \cup \left\{ z \right\}$.
\item
If $P \lts{\tau} Q$ then $\fv{Q} \subseteq \fv{P}$.
\end{itemize}
\end{lemma}
For the applied $\pi$-calculus, the above properties need to be induced as an explicit assumption.

\paragraph{Proposition~\ref{proposition:late}.}
Open bisimilarity is sound with respect to strong equivalence for $\pi$-calculus with mismatch.

\begin{proof}
Suppose that $R \sim S$ 
such that $\fv{R} \cup \fv{S} \subseteq \left\{x_1, \hdots x_n \right\}$.
%, where $m$ is greater than $n$ plus the number of input actions in $P$ and $Q$.
By Theorem~\ref{theorem:congruence},
for $y$ and every distinct $z_1, \ldots, z_m$ such that $\left\{ y, z_1, \ldots, z_m \right\} \cap \left\{x_1, \hdots x_n \right\} = \emptyset$, the following holds:
\[
\nu z_1, \hdots z_m. \co{y}z_1.\hdots \co{y}z_m. y(x_1). \hdots y(x_n). R \sim 
\nu z_1, \hdots z_m. \co{y}z_1.\hdots \co{y}z_m. y(x_1). \hdots y(x_n). S
\]
Hence, for every $m$, by definition of open bisimilarity, there exists open bisimulation $\mathcal{R}_m$ such that the following holds.
\[
\nu z_1, \hdots z_m. \co{y}z_1.\hdots \co{y}z_m. y(x_1). \hdots y(x_n). R
\mathrel{\mathcal{R}_m^{y^i}}
\nu z_1, \hdots z_m. \co{y}z_1.\hdots \co{y}z_m. y(x_1). \hdots y(x_n). S
\]
The union of open bisimulations is an open bisimulation, hence
$\mathrel{R}$, defined as $\bigcup_{m \in \omega} \mathcal{R}_m$, is an open bisimulation.
Since each $\mathcal{R}_m$ is a bisimulation, by closure under transitions, we have
$R \mathrel{\mathcal{R}^{y^i \cdot z_1^o \cdots z^o_m \cdot x_1^i \cdots x_n^i}} S$, for any $m$.
I.e.\ from any open bisimilarity we can construct an open bisimulation for which we can assume an arbirtrary supply of distinct fresh names that we can use to ground messages.

Let $\sigma$ be any substitution such that $\dom{\sigma} \subseteq \left\{ x_1, \hdots x_n \right\}$
and for all $1 \leq i \leq n$ there exists $1 \leq j \leq m$
such that $x_i\sigma = z_j$.
Considering all such substitutions for $n < m$ enforces the law of excluded middle for all variables in $R$ and $S$, since all variables in $R$ and $S$ are either mapped to the same extruded private name or to distinct extruded private names.

It remains to construct a strong equivalence from an open bisimulation.
Given an open bisimulation $\mathcal{R}$ constructed as above, define binary relation $\mathcal{S}$ 
such that:
$P \mathrel{\mathcal{S}} Q$ whenever
$P \mathrel{\mathcal{R}^{h}} Q$ and $h$ grounds $P$ and $Q$.
%is such that all free variables in $P$ and $Q$ 
% in which all variables in $P$ and $Q$ are bound by extruded private names in the history. 
To show that $\mathcal{S}$ defines a late bisimulation,
assume that $P \mathrel{\mathcal{S}} Q$ holds hence
$P \mathrel{\mathcal{R}^{h}} Q$ where $h$ grounds $P$ and $Q$.
%Notice that respectful substitutions and mismatches trivially preserve the fact that $P$ and $Q$ are grounded by the history.
There are three cases to consider, the most interesting being for input transitions.
\begin{itemize}
\item For free outputs and $\tau$ transitions,
Assume $P \lts{\alpha} Q$.
By Lemma~\ref{lemma:transition},
$h \colon P \lts{\alpha} P'$;
hence, there exists $Q'$ such that 
$h \colon Q \lts{\alpha} Q'$ and 
$P' \mathrel{\mathcal{R}^{h}} Q'$.
By Lemma~\ref{lemma:transition}, $Q \lts{\alpha} Q'$.
Furthermore, by Lemma~\ref{lemma:transition-names},
since $\fv{P'} \subseteq \fv{P}$
and
$\fv{Q'} \subseteq \fv{Q}$,
history $h$ grounds $P'$ and $Q'$; hence $P' \mathrel{\mathcal{S}} Q'$.

\item Suppose $P \lts{\co{x}(z)} Q$ 
and $z$ is fresh for $P$, $Q$ and $h$.
By Lemma~\ref{lemma:transition},
$h \colon P \lts{\co{x}(z)} P'$;
hence, there exists $Q'$ such that 
$h \colon Q \lts{\co{x}(z)} Q'$ and 
$P' \mathrel{\mathcal{R}^{h \cdot z^o}} Q'$.
By Lemma~\ref{lemma:transition}, $Q \lts{\co{x}(z)} Q'$.
Furthermore, by Lemma~\ref{lemma:transition-names},
since $\fv{P'} \subseteq \fv{P} \cup \left\{ z \right\}$
and
$\fv{Q'} \subseteq \fv{Q} \cup \left\{ z \right\}$,
history $h \cdot x^o$ grounds $P'$ and $Q'$; hence $P' \mathrel{\mathcal{S}} Q'$.

\item Suppose $P \lts{x(z)} Q$ 
and $z$ is fresh for $P$, $Q$ and $h$.
By Lemma~\ref{lemma:transition},
$h \colon P \lts{x(z)} P'$;
hence, there exists $Q'$ such that 
$h \colon Q \lts{\co{x}(z)} Q'$ and 
$P' \mathrel{\mathcal{R}^{h \cdot z^i}} Q'$.
By Lemma~\ref{lemma:transition}, $Q \lts{\co{x}(z)} Q'$.
Furthermore, 
for all varaibles $w$ appearing as an output in the history $h$,
$\sub{z}{w}$ respects $h \cdot x^i$ and hence
$P'\sub{z}{w} \mathrel{\mathcal{R}^{h \cdot w^i}} Q'\sub{z}{w}$ holds.
Since our construction allows us to assume an arbitrary supply of fresh names in the history, this covers the cases where $w$ is a known free variable, a previously extruded private name or a properly fresh name, as yet unused in the history.
Furthermore, by Lemma~\ref{lemma:transition-names},
since $\fv{P'} \subseteq \fv{P} \cup \left\{ z \right\}$
and
$\fv{Q'} \subseteq \fv{Q} \cup \left\{ z \right\}$,
history $h \cdot w^i$ grounds $P'\sub{z}{w}$ and $Q'\sub{z}{w}$; hence $P' \mathrel{\mathcal{S}} Q'$.
\end{itemize}
Thereby $\mathrel{S}$ is a late bisimulation
such that $R\sigma$ is late bisimilar to $S\sigma$ for any name substitution.
Hence $R$ is strongly equivalent to $S$.
\end{proof}

\subsection{Quasi-open bisimulation}

In the paper, we mention quasi-open bisimulation. Quasi-open bisimulation has received relatively little attention compared to open, late and early bisimulation, hence is only mentioned to highlight important related work in the body of the paper.

Despite its relative lack of attention in the litterature, quasi-open bisimulation is an imporant reference; hence will receive dedicated attention in a separate paper.
\ross{Maybe include definition here.}

For quasi-open bisimulation, what about:
\[
\match{x \not= y}\tau.\match{x = w}\match{y = z}\tau
\not\sim 
\match{x \not= y}\tau
\]
We can try context
 $\contextn{1}{} \triangleq a(w).a(x).\left\{\ \cdot\ \right\} \cpar \nu n.\co{a}n.\co{a}n$.
Clearly,
$
\contextn{1}{\match{x \not= y}\tau.\match{x = w}\match{y = z}\tau}
\lts{\tau} \lts{\tau} 
\nu n.\match{n \not= y}\tau.\match{n = n}\match{y = z}\tau
\lts{\tau} \match{n = n}\match{y = z}\tau
$.
Now given
$\contextn{2}{} \triangleq a(y).\left\{\ \cdot\ \right\} \cpar \co{a}z$,
we have
$\contextn{2}{\match{n = n}\match{y = z}\tau} \lts{\tau} \match{n = n}\match{z = z}\tau$;
and finally $\match{n = n}\match{z = z}\tau \lts{\tau} 0$.
Process 
$\match{x \not= y}\tau$ can march all but the last steps.

What about:
\[
\match{x \not= y}\tau.\left(\match{x = w}\co{w}w + \match{y = z}\co{z}z\right)
\not\sim 
\match{x \not= y}\tau.\match{x = w}\co{w}w
\match{x \not= y}\tau.\match{y = z}\co{z}z
\]

\subsection{Early bisimulation}

In contrast, most previous work on the applied $\pi$-calculus focuses on variants of early bisimulation.
There are only two significant difference in the labelled transition semantics --- when a name is output and when an interaction occurs.
The early rules that differ are provided below for easy comparison with the late rule in Fig.~\ref{figure:active}.
\begin{gather*}
\begin{prooftree}
\justifies
\mathopen{\cin{M}{x}.}P \lts{M\,N} {P}
\end{prooftree}
\qquad\qquad
\begin{prooftree}
A \lts{M\,x} A'
\quad
B \lts{\co{M}(x)} B'
\quad x \not\in\fv{A}
\justifies
{A \cpar B}\lts{\tau}{\mathopen{\nu x.}\left(A' \cpar B'\right)} 
\end{prooftree}
\\[5pt]
\begin{prooftree}
P \lts{M\,x} A
\qquad
P \lts{\co{M}(x)} B
\quad x \not\in\fv{P}
\justifies
\bang P \lts{\tau} \mathopen{\nu x.}\left( A \cpar B \right) \cpar \bang P
\end{prooftree}
\end{gather*}
These rules are exactly as for the standard early and late labelled transition systems for the $\pi$-calculus~\cite{milner93tcs}.
The only difference is that channels and values passed are both permitted to be any message, not only variables.

With respect to the early labelled transition system, early bisimulation can be defined as follows.
\begin{definition}[early bisimulation]
For applied $\pi$-calculus, 
an early bisimulation $\mathcal{R}$ is a symmetric relation over extended processes such that
whenverf $P \mathrel{\mathcal{R}} Q$ we have:
\begin{itemize}
\item $P$ is statically equivalent to $Q$.

\item If $P \lts{\pi} P'$ then there exists $Q'$ such that $Q \lts{\pi} Q'$ and $P' \mathrel{\mathcal{R}} Q'$.
\end{itemize}
\end{definition}
